# Supplementary material for: Linear Response Theory: A Modern Analytic-Algebraic Approach
Source: arXiv:1612.01710 source file (2016-12-06)
Supplement: Supplementary file 1 [file appendix.tex]

\appendix
\section{Modular automorphism group and KMS condition}
Following \cite[Chapter VIII, Section 1]{takesaki-03} let us introduce the following definition.
\begin{definition}[KMS condition]
Let $\Alg$ a von Neumann algebra, equipped with a one-parameter group of automorphisms $\{\sigma_t\}_{t \in \R}$. A (lower semicontinuous) weight $\mathcal{T}$ on $\Alg$ is said to satisfy the \emph{modular} or \emph{KMM condition} for $\{\sigma_t\}_{t \in \R}$ if the following two conditions hold:
\begin{itemize}
\item[(1)] $
\mathcal{T}\;\circ\; \sigma_t = \mathcal{T}
$ for all $t \in \R$;
\vspace{1mm}
\item[(2)] For every pair $A,B \in \mathscr{I}_{\mathcal{T}}\cap\mathscr{I}_{\mathcal{T}}^*$ there exists a bounded continuous function $F_{A,B}:\overline{\Lambda}\to \C$
where $\Lambda:=\{z \in \C\ |\ 0<{\rm Im}(z)<1\}$, which is holomorphic on $\Lambda$ and such that
$$
F_{A,B}(t) = \mathcal{T}\big(\sigma_t(A)B\big), \qquad\quad F_{A,B}(t+ \ii) = \mathcal{T}\big(B\sigma_t(A)\big), \qquad\quad t \in \R. 
$$
\end{itemize} 
A weight $\mathcal{T}$ on $\Alg$ is said to satisfy the \emph{KMM condition}
ad inverse temperature $\beta \in \R$ if $\mathcal{T}$ satisfy the \emph{KMM condition} for $\{\sigma_{-\beta t}\}_{t \in \R}$. 
\end{definition}

\medskip

\begin{theorem}[{{\cite[Chapter VIII, Theorem~1.2]{takesaki-03}}}]
To each weight $\mathcal{T}$ on a von Neumann algebra $\Alg$ there corresponds uniquely a one-parameter group of automorphisms 
$\{\sigma_t^{\mathcal{T}}\}_{t \in \R}$, called the \emph{modular automorphism group}, for which $\mathcal{T}$ satisfies the \emph{KMM condition}. 
\end{theorem}

\noindent If $\mathcal{T}$ is a normal faithful semi-finite trace one has that $\sigma_t^{\mathcal{T}}=\id$ for all $t \in \R$.

\begin{theorem}[{{\cite[Chapter VIII, Theorem~3.14]{takesaki-03}}}]
Let $\Alg$ be a semi-finite von Neumann algebra and $\mathcal{T}$ a normal faithful semi-finite trace on $\Alg$. Let $\CMcal{G}$ be a normal faithful semi-finite weight on $\Alg$. The modular automorphism group $\{\sigma_t^{\CMcal{F}}\}_{t \in \R}$ associated to the 
weight $\CMcal{F}$ is inner in the sense that there exists a strongly continuous unitary group $\{U_t\}_{t \in \R}\subset\Alg$ such that
$\sigma_t^{\CMcal{F}}(A)=U_tAU_t^*$ for all $A \in \Alg$. Moreover, $U_t=h^{it}$ with $h$ a positive, invertible selfadjoint operator affiliated with $\Alg$ (and $H={\log h}$). Finally, $\CMcal{F}$ can be written uniquely in the form
$$
\CMcal{F}(A) = \lim_{\eps \to 0}\; \mathcal{T}(h_{\Phi,\eps}\; A), \qquad\quad A \in \Alg^+
$$
with $h_{\Phi,\eps}:=\frac{h}{(1+\eps h)}$, $\eps > 0$.
\end{theorem}

\section{Regular representations of $\Alg$}

We know from Remark \label{framework:remark:abstract_Hilbert_Schmidt_space} that $\mathfrak{L}^2(\Alg)$ is an Hilbert space and let us denoted with $\mathscr{B}(\mathfrak{L}^2(\Alg))$ the set of the bounded operators acting on $\mathfrak{L}^2(\Alg)$. 
The mapping $\pi_{\rm L}:\Alg\to \mathscr{B}(\mathfrak{L}^2(\Alg))$, defined by $\Alg\ni A\mapsto \pi_{\rm L}(A) \in \mathscr{B}(\mathfrak{L}^2(\Alg))$,
 where the operator $\pi_{\rm L}(A)$ acts as
$$
\pi_{\rm L}(A)[B] := AB, \qquad\quad B \in \mathfrak{L}^2(\Alg)\;
$$
provides a maping of the von Neumann algebra $\Alg$ on $\mathscr{B}(\mathfrak{L}^2(\Alg))$. Let us denote with 
 $\Alg_{\rm L}:=\pi_{\rm L}(\Alg)$ the 
image of $\Alg$ in
$\mathscr{B}(\mathfrak{L}^2(\Alg))$ via $\pi_{\rm L}$. The map 
$\pi_{\rm L}$ turns out to be a $\ast$-isomorphism between the algebras $\Alg$ and $\Alg_{\rm L}$, namely provides a faithful representation of 
$\Alg$ called \emph{left regular representation} (see \eg \cite{potapov-sukochev-07,potapov-sukochev-08}).
The algebra $\Alg_{\rm L}$ is equipped with the n.s.f trace $\mathcal{T}_{\rm L}:=\mathcal{T}\circ \pi_{\rm L}^{-1}$ and with this definition the mapping $\pi_{\rm L}$ becomes a trace preserving $\ast$-isomorphism. Consequently, we can identify $\Alg_{\rm L}\simeq\Alg$ and by an extension of $\pi_{\rm L}$ ($\ast$-homeomorphism of topological $\ast$-algebras) also $\rr{M}(\Alg_{\rm L})\simeq\rr{M}(\Alg)$. We notice that if $A \in \rr{M}(\Alg)$ then $\pi_{\rm L}(A)$ is the unbounded operator with domain $\domain(\pi_{\rm L}(A)):=\{B \in \mathfrak{L}^2(\Alg)\ |\ AB \in \mathfrak{L}^2(\Alg)\}$. In a similar way one can construct the \emph{right regular representation} $\Alg\ni A\mapsto \pi_{\rm R}(A) \in \mathscr{B}(\mathfrak{L}^2(\Alg))$ by
$$
\pi_{\rm R}(A)[B] := BA, \qquad\quad B \in \mathfrak{L}^2(\Alg)\;
$$
and the corresponding $\ast$-isomorphic images $\Alg_{\rm R}\simeq\Alg$ and $\rr{M}(\Alg_{\rm R})\simeq\rr{M}(\Alg)$.
